# Supplementary material for: ConeQuest: A Benchmark for Cone Segmentation on Mars
Source: arXiv:2311.08657 source file (2023-11-15)
Supplement: Supplementary file 1 [file trial.tex]

\begin{table*}[!hbt]
\setlength\tabcolsep{4.0pt}
\setlength{\belowcaptionskip}{-10pt}
\centering
\footnotesize
\resizebox{0.96\linewidth}{!}{
\begin{tabular}{c|c|c|ccccccccc|c}
\toprule[1.5pt]
\multirow{2}{*}{\textbf{\begin{tabular}[c]{@{}c@{}}Training\\Category\end{tabular}}} &
  \multirow{2}{*}{\textbf{\begin{tabular}[c]{@{}c@{}}Testing\\Category\end{tabular}}} &
  \multicolumn{1}{l|}{\multirow{2}{*}{\textbf{\begin{tabular}[c]{@{}l@{}}Training\\Model\end{tabular}}}} &
  \multicolumn{9}{c|}{\textbf{Cone}} &
  \textbf{Non-cone} \\ \cmidrule{4-13}
 &
   &
  \multicolumn{1}{l|}{} &
  \multicolumn{1}{c|}{\textbf{\begin{tabular}[c]{@{}c@{}}Pixel\\IoU\end{tabular}}} &
  \multicolumn{1}{c|}{\textbf{\begin{tabular}[c]{@{}c@{}}Pixel\\Accuracy\end{tabular}}} &
  \multicolumn{1}{c|}{\textbf{\begin{tabular}[c]{@{}c@{}}Pixel\\Precision\end{tabular}}} &
  \multicolumn{1}{c|}{\textbf{\begin{tabular}[c]{@{}c@{}}Pixel\\Recall\end{tabular}}} &
  \multicolumn{1}{c|}{\textbf{mAP}} &
  \multicolumn{1}{c|}{\textbf{\begin{tabular}[c]{@{}c@{}}Object\\IoU\end{tabular}}} &
  \multicolumn{1}{c|}{\textbf{\begin{tabular}[c]{@{}c@{}}Object\\Accuracy\end{tabular}}} &
  \multicolumn{1}{c|}{\textbf{\begin{tabular}[c]{@{}c@{}}Object\\Precision\end{tabular}}} &
  \textbf{\begin{tabular}[c]{@{}c@{}}Object\\Recall\end{tabular}} &
  $A_{FP}$ \\ \midrule
&
  \cellcolor[HTML]{FBB982} &
  U-Net &
  \multicolumn{1}{c|}{30.85} &
  \multicolumn{1}{c|}{97.84} &
  \multicolumn{1}{c|}{79.57} &
  \multicolumn{1}{c|}{37.36} &
  \multicolumn{1}{c|}{14.14} &
  \multicolumn{1}{c|}{30.52} &
  \multicolumn{1}{c|}{25.34} &
  \multicolumn{1}{c|}{34.08} &
  28.33 &
  0.25 \\
 &
  \cellcolor[HTML]{FBB982} &
  FPN &
  \multicolumn{1}{c|}{23.97} &
  \multicolumn{1}{c|}{97.53} &
  \multicolumn{1}{c|}{82.85} &
  \multicolumn{1}{c|}{28.39} &
  \multicolumn{1}{c|}{7.42} &
  \multicolumn{1}{c|}{24.44} &
  \multicolumn{1}{c|}{19.53} &
  \multicolumn{1}{c|}{27.48} &
  22.46 &
  0.13 \\
 &
  \cellcolor[HTML]{FBB982} &
  DeepLab &
  \multicolumn{1}{c|}{25.68} &
  \multicolumn{1}{c|}{97.77} &
  \multicolumn{1}{c|}{85.34} &
  \multicolumn{1}{c|}{30.06} &
  \multicolumn{1}{c|}{11.67} &
  \multicolumn{1}{c|}{24.85} &
  \multicolumn{1}{c|}{20.63} &
  \multicolumn{1}{c|}{27.25} &
  24.85 &
  0.03 \\
 &
  \multirow{-4}{*}{\cellcolor[HTML]{FBB982}S} &
  MA-Net &
  \multicolumn{1}{c|}{37.39} &
  \multicolumn{1}{c|}{97.52} &
  \multicolumn{1}{c|}{62.84} &
  \multicolumn{1}{c|}{54.41} &
  \multicolumn{1}{c|}{14.21} &
  \multicolumn{1}{c|}{41.84} &
  \multicolumn{1}{c|}{30.58} &
  \multicolumn{1}{c|}{38.42} &
  41.57 &
  0.42 \\ \cmidrule{2-13} 
 &
  \cellcolor[HTML]{FBB982} &
  U-Net &
  \multicolumn{1}{c|}{41.88} &
  \multicolumn{1}{c|}{93.27} &
  \multicolumn{1}{c|}{85.45} &
  \multicolumn{1}{c|}{47.18} &
  \multicolumn{1}{c|}{19.15} &
  \multicolumn{1}{c|}{48.00} &
  \multicolumn{1}{c|}{41.69} &
  \multicolumn{1}{c|}{54.05} &
  46.08 &
  0.50 \\
 &
  \cellcolor[HTML]{FBB982} &
  FPN &
  \multicolumn{1}{c|}{33.26} &
  \multicolumn{1}{c|}{92.22} &
  \multicolumn{1}{c|}{84.74} &
  \multicolumn{1}{c|}{37.58} &
  \multicolumn{1}{c|}{13.15} &
  \multicolumn{1}{c|}{39.57} &
  \multicolumn{1}{c|}{32.25} &
  \multicolumn{1}{c|}{42.61} &
  37.31 &
  0.26 \\
 &
  \cellcolor[HTML]{FBB982} &
  DeepLab &
  \multicolumn{1}{c|}{28.14} &
  \multicolumn{1}{c|}{91.80} &
  \multicolumn{1}{c|}{91.75} &
  \multicolumn{1}{c|}{30.26} &
  \multicolumn{1}{c|}{11.96} &
  \multicolumn{1}{c|}{29.31} &
  \multicolumn{1}{c|}{24.94} &
  \multicolumn{1}{c|}{31.90} &
  28.41 &
  0.07 \\
 &
  \multirow{-4}{*}{\cellcolor[HTML]{FBB982}M} &
  MA-Net &
  \multicolumn{1}{c|}{50.88} &
  \multicolumn{1}{c|}{94.06} &
  \multicolumn{1}{c|}{81.20} &
  \multicolumn{1}{c|}{61.02} &
  \multicolumn{1}{c|}{18.00} &
  \multicolumn{1}{c|}{55.60} &
  \multicolumn{1}{c|}{43.67} &
  \multicolumn{1}{c|}{50.20} &
  56.56 &
  0.55 \\ \cmidrule{2-13} 
 &
   &
  U-Net &
  \multicolumn{1}{c|}{29.9} &
  \multicolumn{1}{c|}{82.65} &
  \multicolumn{1}{c|}{92.01} &
  \multicolumn{1}{c|}{31.07} &
  \multicolumn{1}{c|}{14.53} &
  \multicolumn{1}{c|}{33.21} &
  \multicolumn{1}{c|}{29.35} &
  \multicolumn{1}{c|}{34.88} &
  34.56 &
  0.05 \\
 &
   &
  FPN &
  \multicolumn{1}{c|}{22.83} &
  \multicolumn{1}{c|}{81.06} &
  \multicolumn{1}{c|}{93.26} &
  \multicolumn{1}{c|}{23.51} &
  \multicolumn{1}{c|}{10.72} &
  \multicolumn{1}{c|}{22.56} &
  \multicolumn{1}{c|}{22.63} &
  \multicolumn{1}{c|}{25.61} &
  25.61 &
  0.09 \\
 &
   &
  DeepLab &
  \multicolumn{1}{c|}{16.48} &
  \multicolumn{1}{c|}{79.34} &
  \multicolumn{1}{c|}{93.39} &
  \multicolumn{1}{c|}{16.83} &
  \multicolumn{1}{c|}{8.42} &
  \multicolumn{1}{c|}{19.94} &
  \multicolumn{1}{c|}{16.45} &
  \multicolumn{1}{c|}{20.44} &
  19.95 &
  0.05 \\
\multirow{-12}{*}{S + M} &
  \multirow{-4}{*}{L} &
  MA-Net &
  \multicolumn{1}{c|}{51.11} &
  \multicolumn{1}{c|}{86.35} &
  \multicolumn{1}{c|}{90.39} &
  \multicolumn{1}{c|}{56.31} &
  \multicolumn{1}{c|}{18.89} &
  \multicolumn{1}{c|}{53.78} &
  \multicolumn{1}{c|}{44.56} &
  \multicolumn{1}{c|}{48.19} &
  63.07 &
  0.33 \\ \midrule
 &
   &
  U-Net &
  \multicolumn{1}{c|}{23.63} &
  \multicolumn{1}{c|}{96.83} &
  \multicolumn{1}{c|}{69.32} &
  \multicolumn{1}{c|}{30.29} &
  \multicolumn{1}{c|}{7.37} &
  \multicolumn{1}{c|}{21.23} &
  \multicolumn{1}{c|}{16.79} &
  \multicolumn{1}{c|}{24.06} &
  18.68 &
  1.00 \\
 &
   &
  FPN &
  \multicolumn{1}{c|}{19.01} &
  \multicolumn{1}{c|}{96.60} &
  \multicolumn{1}{c|}{73.26} &
  \multicolumn{1}{c|}{25.05} &
  \multicolumn{1}{c|}{7.23} &
  \multicolumn{1}{c|}{15.24} &
  \multicolumn{1}{c|}{8.94} &
  \multicolumn{1}{c|}{14.33} &
  11.87 &
  0.65 \\
 &
   &
  DeepLab &
  \multicolumn{1}{c|}{17.24} &
  \multicolumn{1}{c|}{96.95} &
  \multicolumn{1}{c|}{80.52} &
  \multicolumn{1}{c|}{21.44} &
  \multicolumn{1}{c|}{8.26} &
  \multicolumn{1}{c|}{15.60} &
  \multicolumn{1}{c|}{11.16} &
  \multicolumn{1}{c|}{16.74} &
  12.87 &
  1.06 \\
 &
  \multirow{-4}{*}{S} &
  MA-Net &
  \multicolumn{1}{c|}{22.42} &
  \multicolumn{1}{c|}{97.02} &
  \multicolumn{1}{c|}{76.47} &
  \multicolumn{1}{c|}{28.04} &
  \multicolumn{1}{c|}{6.36} &
  \multicolumn{1}{c|}{21.96} &
  \multicolumn{1}{c|}{15.71} &
  \multicolumn{1}{c|}{23.10} &
  17.55 &
  0.81 \\ \cmidrule{2-13} 
 &
  \cellcolor[HTML]{FBB982} &
  U-Net &
  \multicolumn{1}{c|}{46.28} &
  \multicolumn{1}{c|}{92.98} &
  \multicolumn{1}{c|}{75.76} &
  \multicolumn{1}{c|}{55.25} &
  \multicolumn{1}{c|}{14.89} &
  \multicolumn{1}{c|}{48.40} &
  \multicolumn{1}{c|}{37.85} &
  \multicolumn{1}{c|}{50.29} &
  43.68 &
  0.70 \\
 &
  \cellcolor[HTML]{FBB982} &
  FPN &
  \multicolumn{1}{c|}{40.52} &
  \multicolumn{1}{c|}{92.56} &
  \multicolumn{1}{c|}{76.16} &
  \multicolumn{1}{c|}{48.22} &
  \multicolumn{1}{c|}{15.70} &
  \multicolumn{1}{c|}{41.77} &
  \multicolumn{1}{c|}{31.19} &
  \multicolumn{1}{c|}{42.90} &
  36.84 &
  0.48 \\
 &
  \cellcolor[HTML]{FBB982} &
  DeepLab &
  \multicolumn{1}{c|}{40.49} &
  \multicolumn{1}{c|}{92.49} &
  \multicolumn{1}{c|}{81.37} &
  \multicolumn{1}{c|}{47.06} &
  \multicolumn{1}{c|}{10.12} &
  \multicolumn{1}{c|}{44.56} &
  \multicolumn{1}{c|}{31.98} &
  \multicolumn{1}{c|}{43.67} &
  37.41 &
  0.51 \\
 &
  \multirow{-4}{*}{\cellcolor[HTML]{FBB982}M} &
  MA-Net &
  \multicolumn{1}{c|}{41.96} &
  \multicolumn{1}{c|}{92.71} &
  \multicolumn{1}{c|}{82.85} &
  \multicolumn{1}{c|}{48.76} &
  \multicolumn{1}{c|}{14.89} &
  \multicolumn{1}{c|}{45.75} &
  \multicolumn{1}{c|}{36.98} &
  \multicolumn{1}{c|}{50.01} &
  41.83 &
  0.33 \\ \cmidrule{2-13} 
 &
  \cellcolor[HTML]{FBB982} &
  U-Net &
  \multicolumn{1}{c|}{52.92} &
  \multicolumn{1}{c|}{88.97} &
  \multicolumn{1}{c|}{88.46} &
  \multicolumn{1}{c|}{58.01} &
  \multicolumn{1}{c|}{17.20} &
  \multicolumn{1}{c|}{53.63} &
  \multicolumn{1}{c|}{47.05} &
  \multicolumn{1}{c|}{53.07} &
  58.56 &
  2.57 \\
 &
  \cellcolor[HTML]{FBB982} &
  FPN &
  \multicolumn{1}{c|}{53.70} &
  \multicolumn{1}{c|}{88.67} &
  \multicolumn{1}{c|}{88.55} &
  \multicolumn{1}{c|}{59.06} &
  \multicolumn{1}{c|}{17.94} &
  \multicolumn{1}{c|}{54.81} &
  \multicolumn{1}{c|}{48.26} &
  \multicolumn{1}{c|}{56.02} &
  57.57 &
  2.88 \\
 &
  \cellcolor[HTML]{FBB982} &
  DeepLab &
  \multicolumn{1}{c|}{64.01} &
  \multicolumn{1}{c|}{91.55} &
  \multicolumn{1}{c|}{91.58} &
  \multicolumn{1}{c|}{69.28} &
  \multicolumn{1}{c|}{23.65} &
  \multicolumn{1}{c|}{65.89} &
  \multicolumn{1}{c|}{56.61} &
  \multicolumn{1}{c|}{63.98} &
  68.73 &
  2.31 \\
\multirow{-12}{*}{M + L} &
  \multirow{-4}{*}{\cellcolor[HTML]{FBB982}L} &
  MA-Net &
  \multicolumn{1}{c|}{60.06} &
  \multicolumn{1}{c|}{90.42} &
  \multicolumn{1}{c|}{92.17} &
  \multicolumn{1}{c|}{64.18} &
  \multicolumn{1}{c|}{23.54} &
  \multicolumn{1}{c|}{61.74} &
  \multicolumn{1}{c|}{57.25} &
  \multicolumn{1}{c|}{63.24} &
  67.13 &
  1.76 \\ \midrule
 &
  \cellcolor[HTML]{FBB982} &
  U-Net &
  \multicolumn{1}{c|}{14.35} &
  \multicolumn{1}{c|}{97.02} &
  \multicolumn{1}{c|}{84.55} &
  \multicolumn{1}{c|}{18.09} &
  \multicolumn{1}{c|}{5.1} &
  \multicolumn{1}{c|}{12.39} &
  \multicolumn{1}{c|}{9.14} &
  \multicolumn{1}{c|}{14.34} &
  10.32 &
  0.93 \\
 &
  \cellcolor[HTML]{FBB982} &
  FPN &
  \multicolumn{1}{c|}{24.01} &
  \multicolumn{1}{c|}{97.28} &
  \multicolumn{1}{c|}{81.13} &
  \multicolumn{1}{c|}{32.41} &
  \multicolumn{1}{c|}{6.93} &
  \multicolumn{1}{c|}{23.82} &
  \multicolumn{1}{c|}{18.47} &
  \multicolumn{1}{c|}{24.34} &
  23.08 &
  0.48 \\
 &
  \cellcolor[HTML]{FBB982} &
  DeepLab &
  \multicolumn{1}{c|}{18.95} &
  \multicolumn{1}{c|}{97.22} &
  \multicolumn{1}{c|}{82.84} &
  \multicolumn{1}{c|}{22.90} &
  \multicolumn{1}{c|}{5.53} &
  \multicolumn{1}{c|}{17.85} &
  \multicolumn{1}{c|}{13.49} &
  \multicolumn{1}{c|}{19.31} &
  16.04 &
  1.19 \\
 &
  \multirow{-4}{*}{\cellcolor[HTML]{FBB982}S} &
  MA-Net &
  \multicolumn{1}{c|}{31.44} &
  \multicolumn{1}{c|}{97.16} &
  \multicolumn{1}{c|}{65.87} &
  \multicolumn{1}{c|}{45.44} &
  \multicolumn{1}{c|}{7.33} &
  \multicolumn{1}{c|}{31.66} &
  \multicolumn{1}{c|}{22.91} &
  \multicolumn{1}{c|}{27.81} &
  33.09 &
  0.95 \\ \cmidrule{2-13} 
 &
   &
  U-Net &
  \multicolumn{1}{c|}{35.82} &
  \multicolumn{1}{c|}{92.78} &
  \multicolumn{1}{c|}{86.03} &
  \multicolumn{1}{c|}{40.87} &
  \multicolumn{1}{c|}{9.83} &
  \multicolumn{1}{c|}{35.77} &
  \multicolumn{1}{c|}{26.82} &
  \multicolumn{1}{c|}{37.47} &
  29.91 &
  0.38 \\
 &
   &
  FPN &
  \multicolumn{1}{c|}{37.05} &
  \multicolumn{1}{c|}{92.63} &
  \multicolumn{1}{c|}{85.55} &
  \multicolumn{1}{c|}{42.08} &
  \multicolumn{1}{c|}{12.42} &
  \multicolumn{1}{c|}{40.55} &
  \multicolumn{1}{c|}{34.11} &
  \multicolumn{1}{c|}{44.38} &
  39.48 &
  0.20 \\
 &
   &
  DeepLab &
  \multicolumn{1}{c|}{34.30} &
  \multicolumn{1}{c|}{92.10} &
  \multicolumn{1}{c|}{81.33} &
  \multicolumn{1}{c|}{40.50} &
  \multicolumn{1}{c|}{8.11} &
  \multicolumn{1}{c|}{36.56} &
  \multicolumn{1}{c|}{23.43} &
  \multicolumn{1}{c|}{30.83} &
  29.79 &
  0.31 \\
 &
  \multirow{-4}{*}{M} &
  MA-Net &
  \multicolumn{1}{c|}{50.29} &
  \multicolumn{1}{c|}{92.94} &
  \multicolumn{1}{c|}{75.99} &
  \multicolumn{1}{c|}{63.65} &
  \multicolumn{1}{c|}{16.41} &
  \multicolumn{1}{c|}{55.66} &
  \multicolumn{1}{c|}{37.56} &
  \multicolumn{1}{c|}{45.75} &
  53.47 &
  0.23 \\ \cmidrule{2-13} 
 &
  \cellcolor[HTML]{FBB982} &
  U-Net &
  \multicolumn{1}{c|}{52.01} &
  \multicolumn{1}{c|}{89.13} &
  \multicolumn{1}{c|}{91.55} &
  \multicolumn{1}{c|}{56.26} &
  \multicolumn{1}{c|}{21.49} &
  \multicolumn{1}{c|}{52.84} &
  \multicolumn{1}{c|}{49.93} &
  \multicolumn{1}{c|}{58.67} &
  56.8 &
  2.22 \\
 &
  \cellcolor[HTML]{FBB982} &
  FPN &
  \multicolumn{1}{c|}{53.22} &
  \multicolumn{1}{c|}{88.22} &
  \multicolumn{1}{c|}{87.40} &
  \multicolumn{1}{c|}{60.37} &
  \multicolumn{1}{c|}{20.24} &
  \multicolumn{1}{c|}{51.47} &
  \multicolumn{1}{c|}{45.58} &
  \multicolumn{1}{c|}{50.81} &
  55.73 &
  1.40 \\
 &
  \cellcolor[HTML]{FBB982} &
  DeepLab &
  \multicolumn{1}{c|}{57.35} &
  \multicolumn{1}{c|}{89.76} &
  \multicolumn{1}{c|}{86.88} &
  \multicolumn{1}{c|}{64.73} &
  \multicolumn{1}{c|}{14.86} &
  \multicolumn{1}{c|}{52.72} &
  \multicolumn{1}{c|}{44.78} &
  \multicolumn{1}{c|}{49.30} &
  57.57 &
  2.36 \\
\multirow{-12}{*}{S + L} &
  \multirow{-4}{*}{\cellcolor[HTML]{FBB982}L} &
  MA-Net &
  \multicolumn{1}{c|}{62.65} &
  \multicolumn{1}{c|}{90.80} &
  \multicolumn{1}{c|}{84.17} &
  \multicolumn{1}{c|}{71.61} &
  \multicolumn{1}{c|}{14.74} &
  \multicolumn{1}{c|}{59.74} &
  \multicolumn{1}{c|}{49.18} &
  \multicolumn{1}{c|}{52.64} &
  67.89 &
  2.50 \\ \bottomrule
\end{tabular}
}
\caption{Results for BM-2 on $\mathcal{D}_{seen}$ (\textit{highlighted}) and $\mathcal{D}_{unseen}$ for multi-category $\mathcal{T}_{pn}$.}
\label{tab:bm_2_multi_all_results}
\end{table*}
